# Supplementary material for: Modeling Behavioral Intensity and Transitions for Generative Recommendation
Source: arXiv:2604.24472 source file (2026-04-27)
Supplement: Supplementary file 1 [file Appendix.tex]

\appendix

\section{Appendix}
